# Supplementary material for: DeFiGuard: A Price Manipulation Detection Service in DeFi using Graph Neural Networks
Source: arXiv:2406.11157 source file (2024-06-17)
Supplement: Supplementary file 1 [file appendix.tex]

\appendix

\begin{figure*}[ht]
    \centering
    \includegraphics[width=1\linewidth]{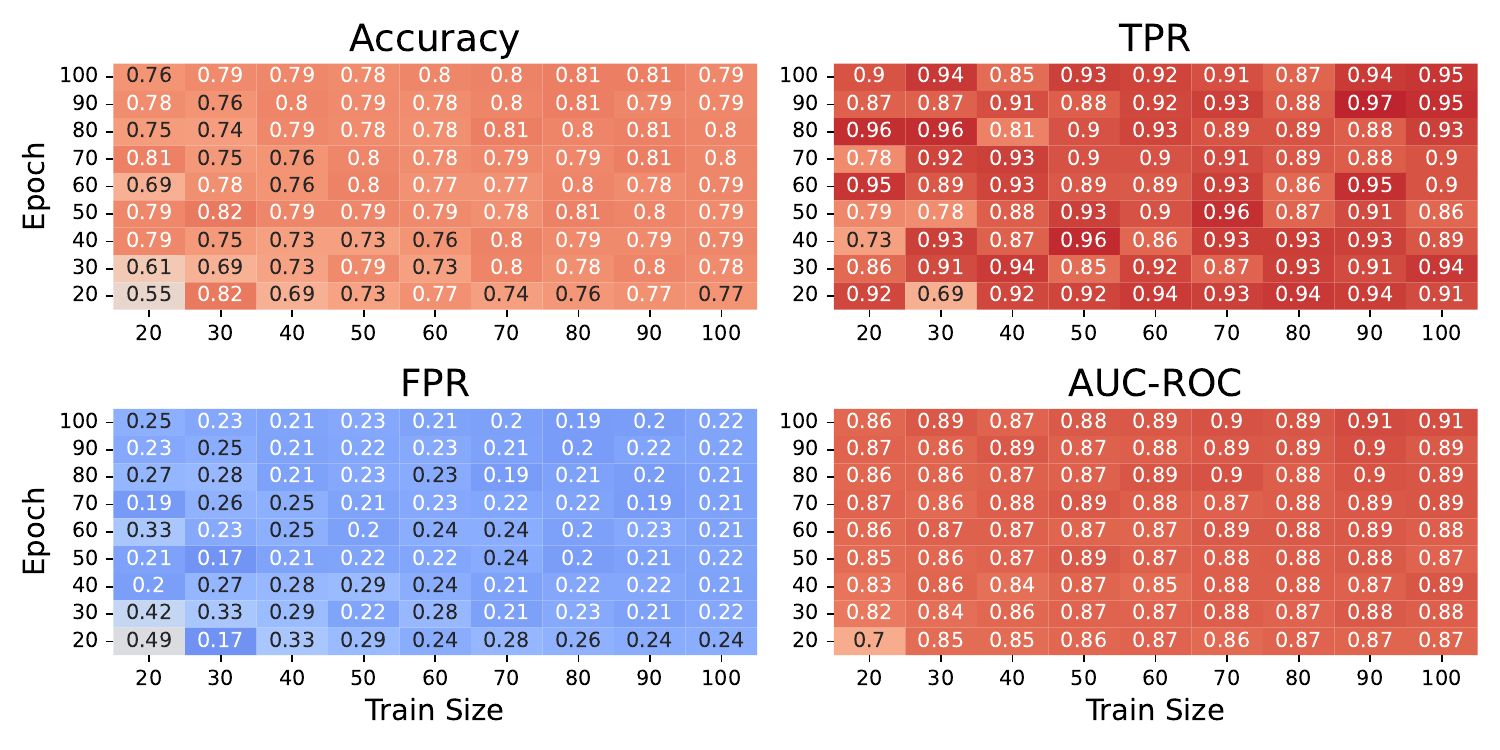}
    \caption{\bf The detailed performance of GCN.} 
    \label{fig:perf_gcn}
\end{figure*}

\begin{figure*}[ht]
    \centering
    \includegraphics[width=1\linewidth]{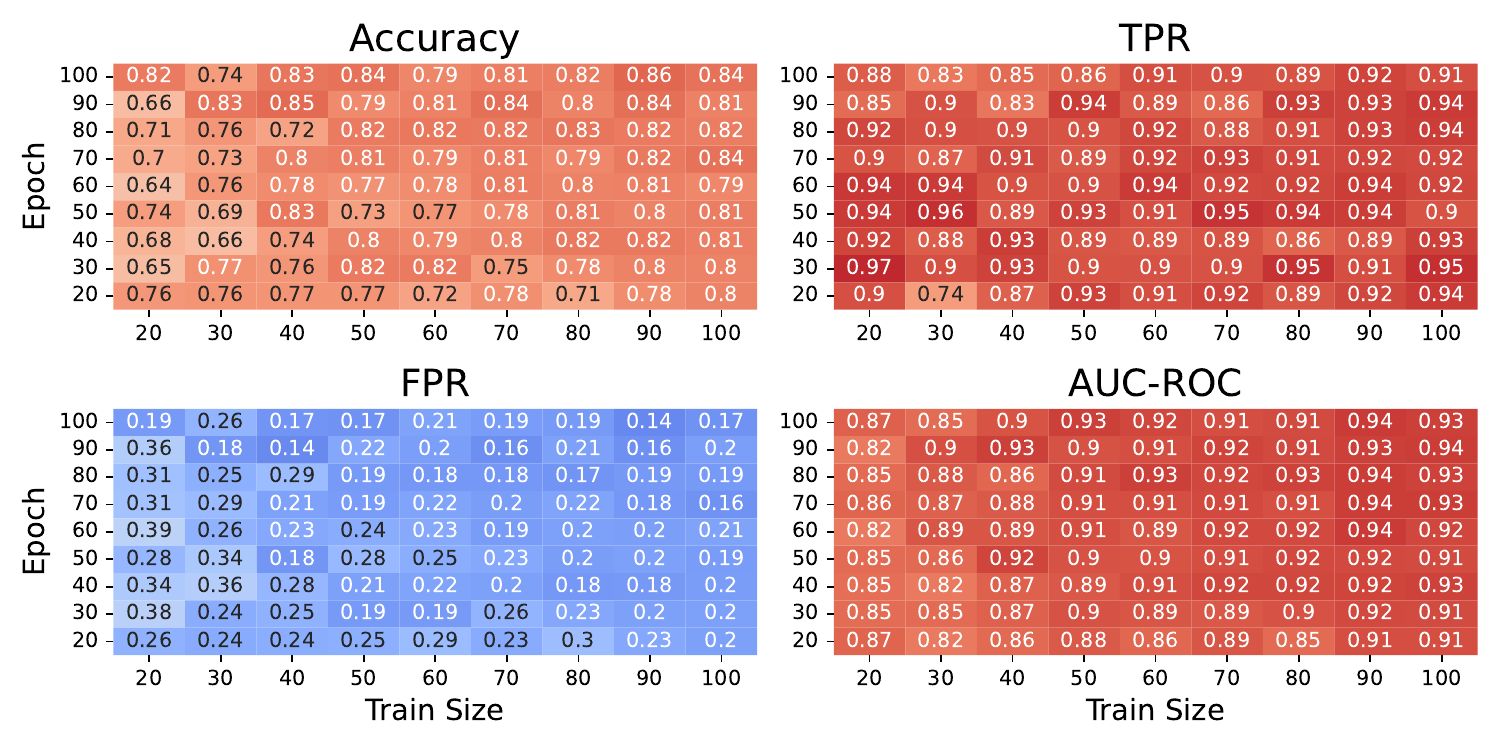}
    \caption{\bf The detailed performance of GAT.} 
    \label{fig:perf_gat}
\end{figure*}

\begin{figure*}[ht]
    \centering
    \includegraphics[width=1\linewidth]{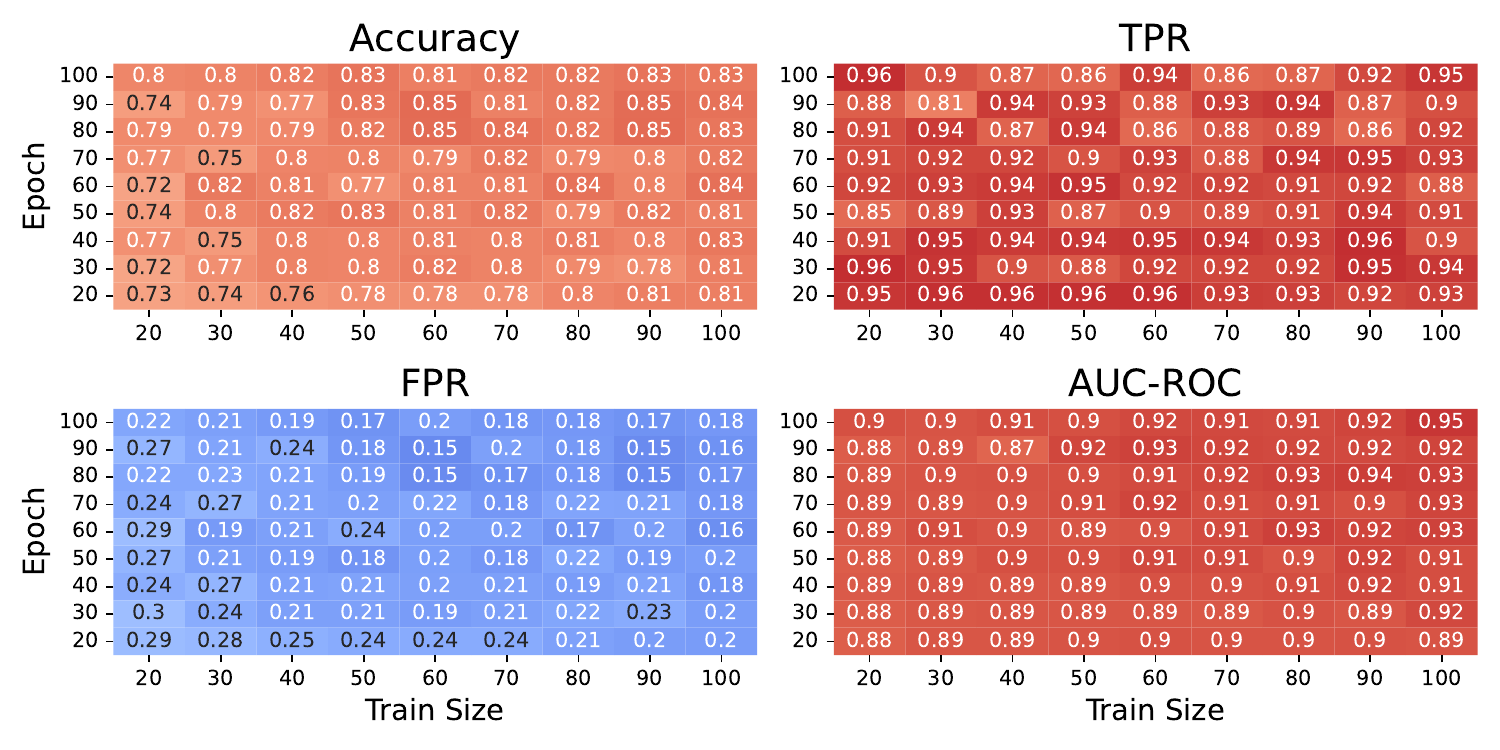}
    \caption{\bf The detailed performance of GIN.} 
    \label{fig:perf_gin}
\end{figure*}

\begin{figure*}[ht]
    \centering
    \includegraphics[width=1\linewidth]{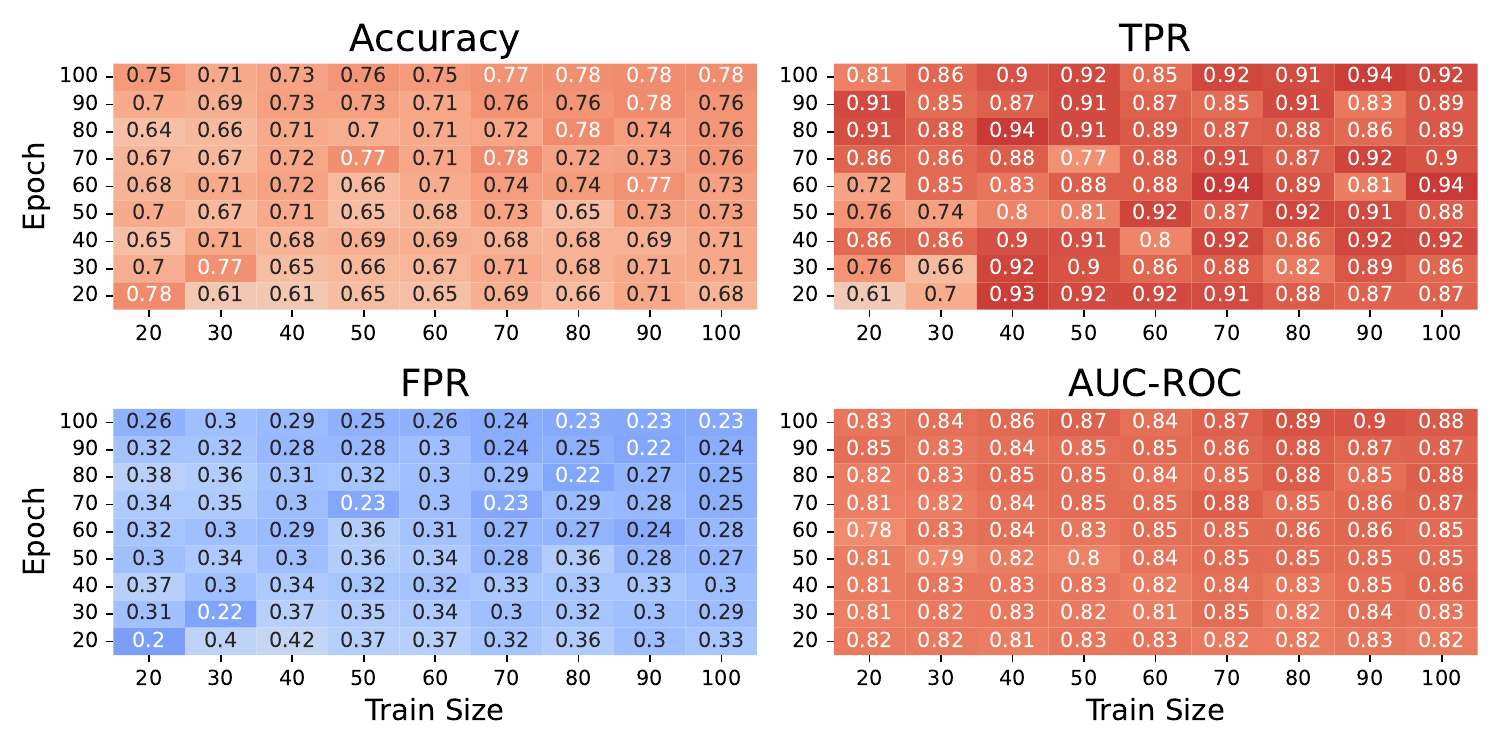}
    \caption{\bf The detailed performance of MLP.} 
    \label{fig:perf_mlp}
\end{figure*}

% \section{Ablation Studies}
% \label{appendix:ablation}

% Figures~\ref{fig:ablation_gat}~\ref{fig:ablation_gin}~\ref{fig:ablation_gcn}~\ref{fig:ablation_mlp} depict the ablation studies using GAT, GCN, GIN, and MLP models.

\begin{figure}[t]
    \centering
    \includegraphics[width=0.9\linewidth]{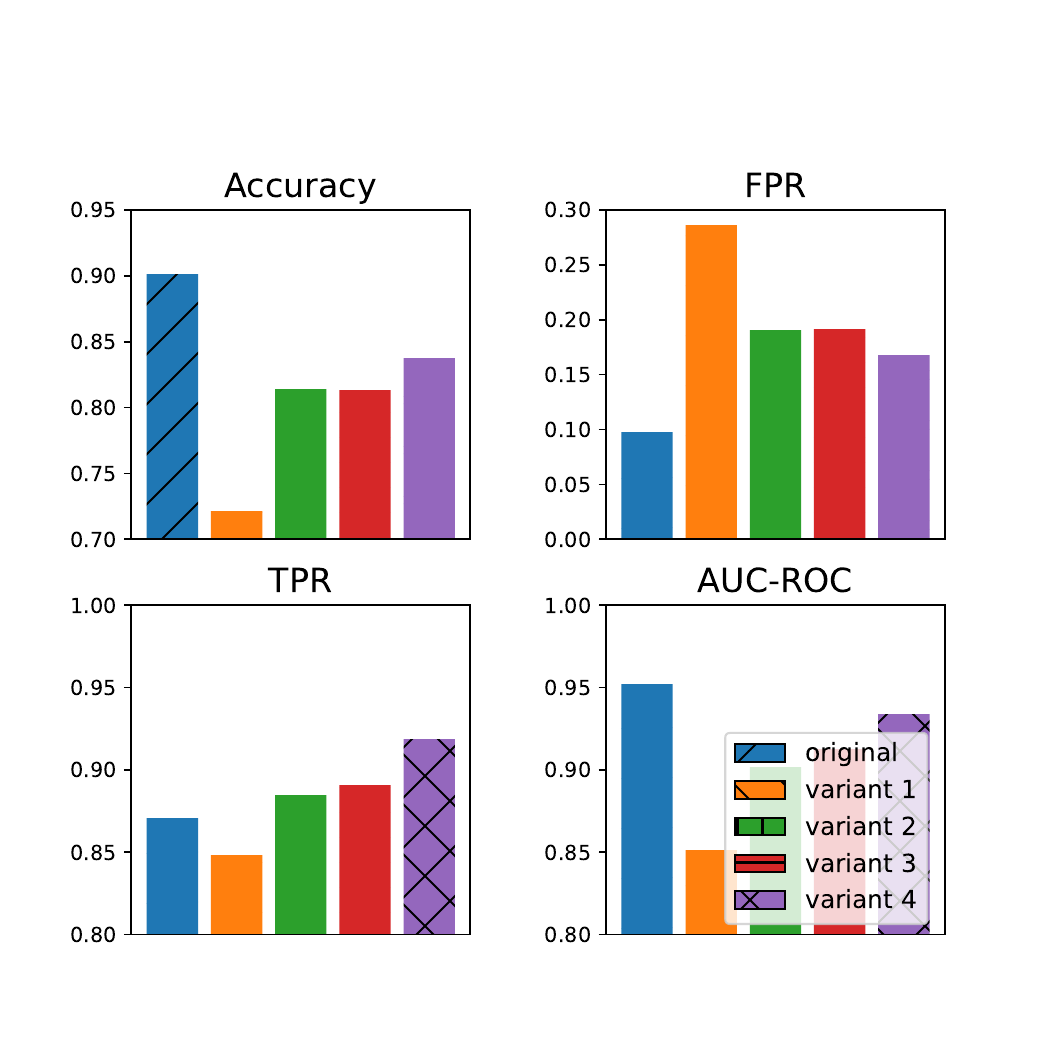}
    \caption{\bf Ablation study with GAT model.} 
    \label{fig:ablation_gat}
\end{figure}

\begin{figure}[t]
    \centering
    \includegraphics[width=0.9\linewidth]{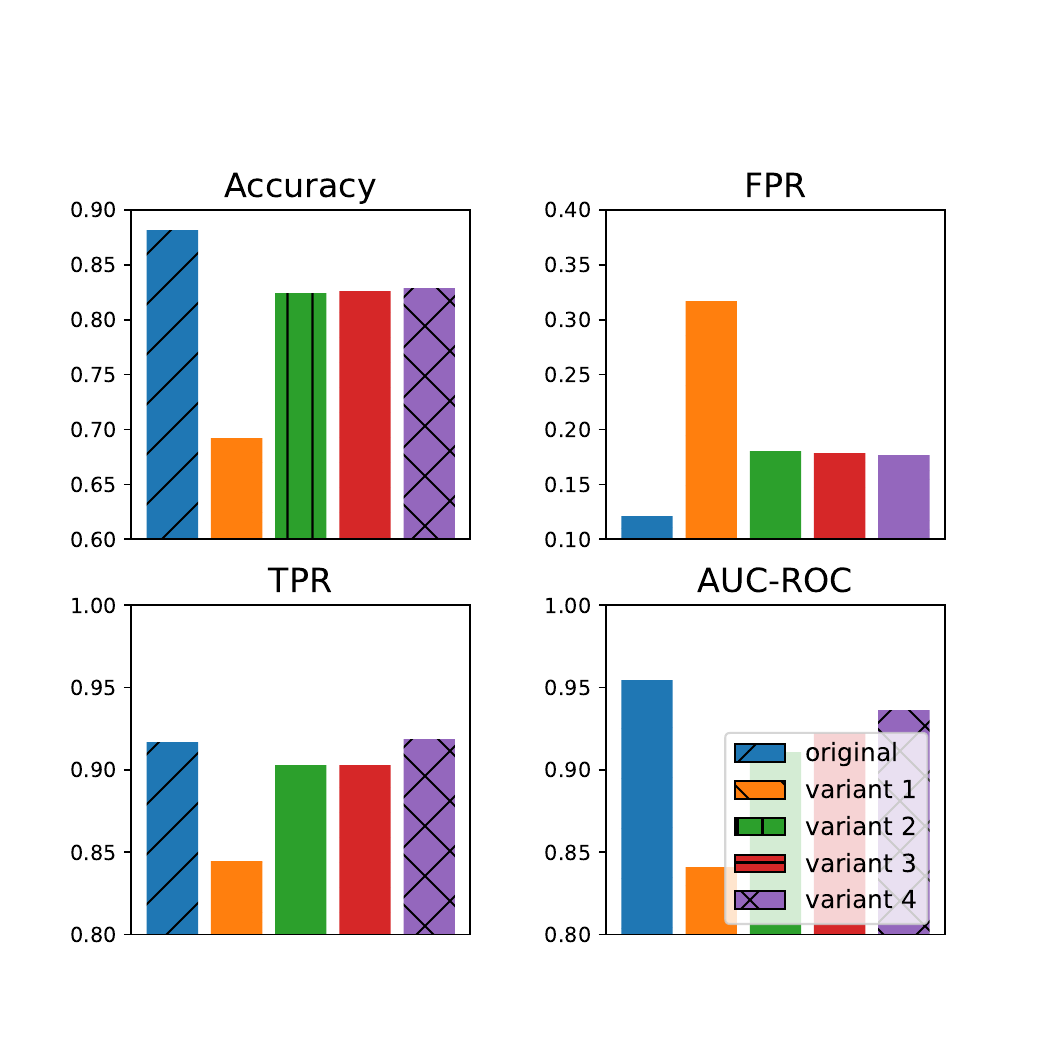}
    \caption{\bf Ablation study with GIN model.} 
    \label{fig:ablation_gin}
\end{figure}

\begin{figure}[t]
    \centering
    \includegraphics[width=0.9\linewidth]{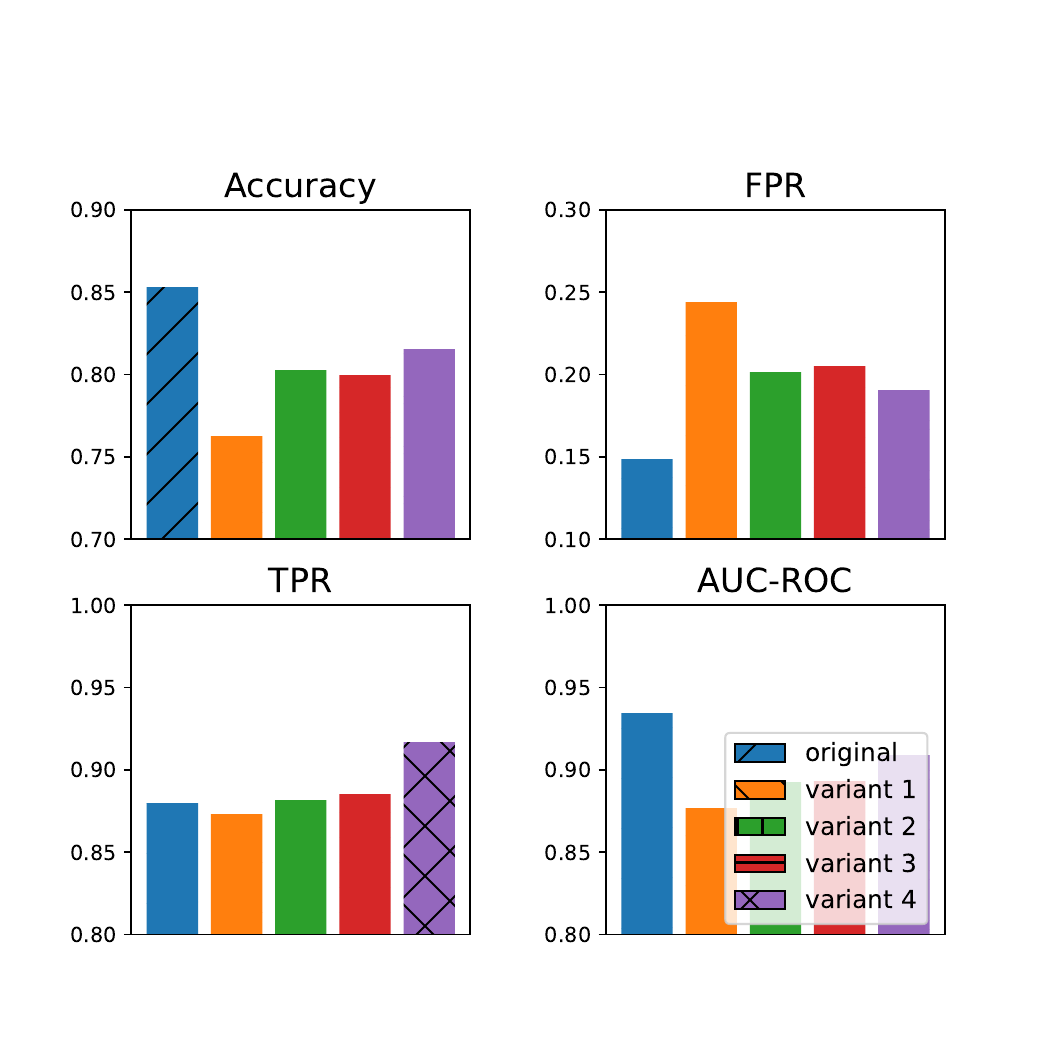}
    \caption{\bf Ablation study with GCN model.} 
    \label{fig:ablation_gcn}
\end{figure}

\begin{figure}[t]
    \centering
    \includegraphics[width=0.9\linewidth]{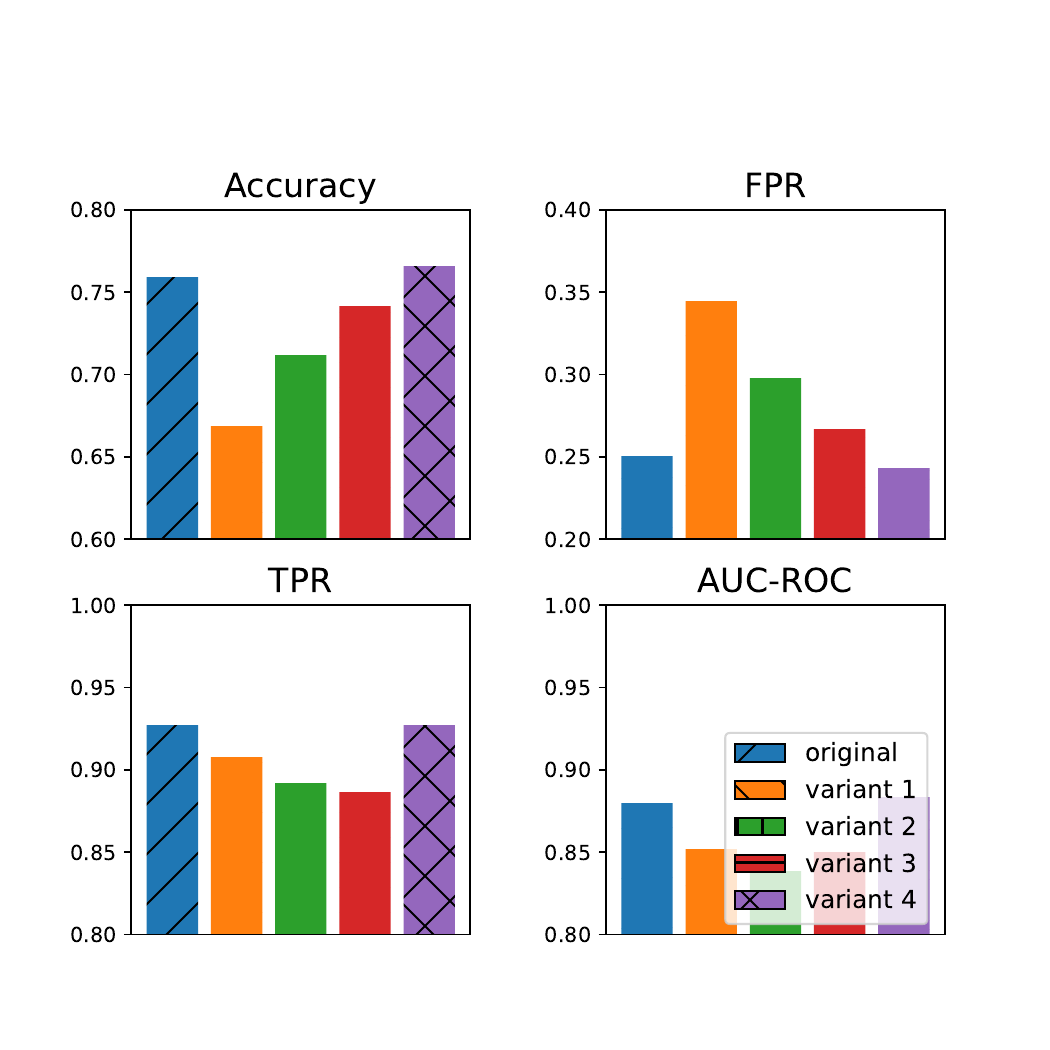}
    \caption{\bf Ablation study with MLP model.} 
    \label{fig:ablation_mlp}
\end{figure}
