# Supplementary material for: DeFiGuard: A Price Manipulation Detection Service in DeFi using Graph Neural Networks
Source: arXiv:2406.11157 source file (2024-06-17)
Supplement: Supplementary file 2 [file appendix_ablation.tex]

\begin{figure}[t]
    \centering
    \includegraphics[width=0.9\linewidth]{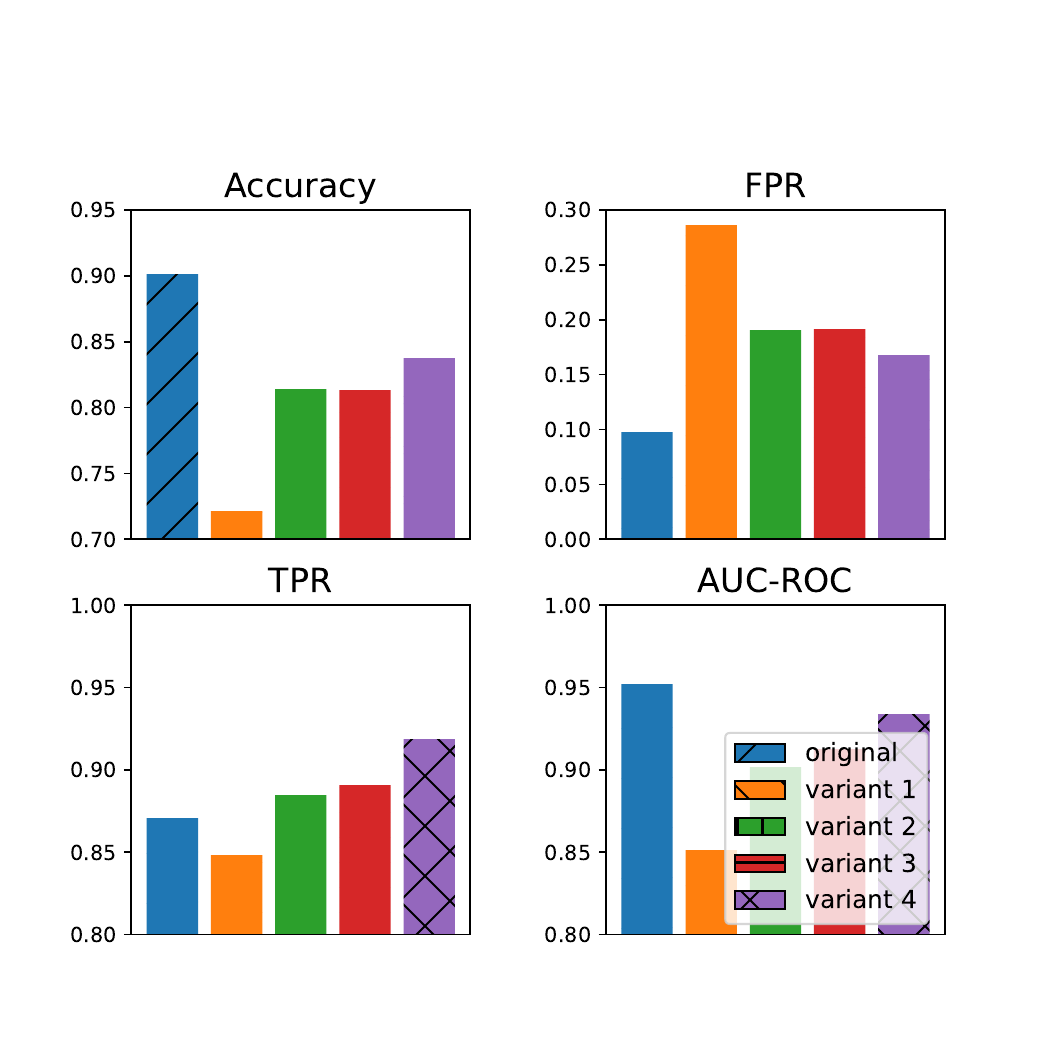}
    \caption{\bf Ablation study with GAT model.} 
    \label{fig:ablation_gat}
\end{figure}

\begin{figure}[t]
    \centering
    \includegraphics[width=0.9\linewidth]{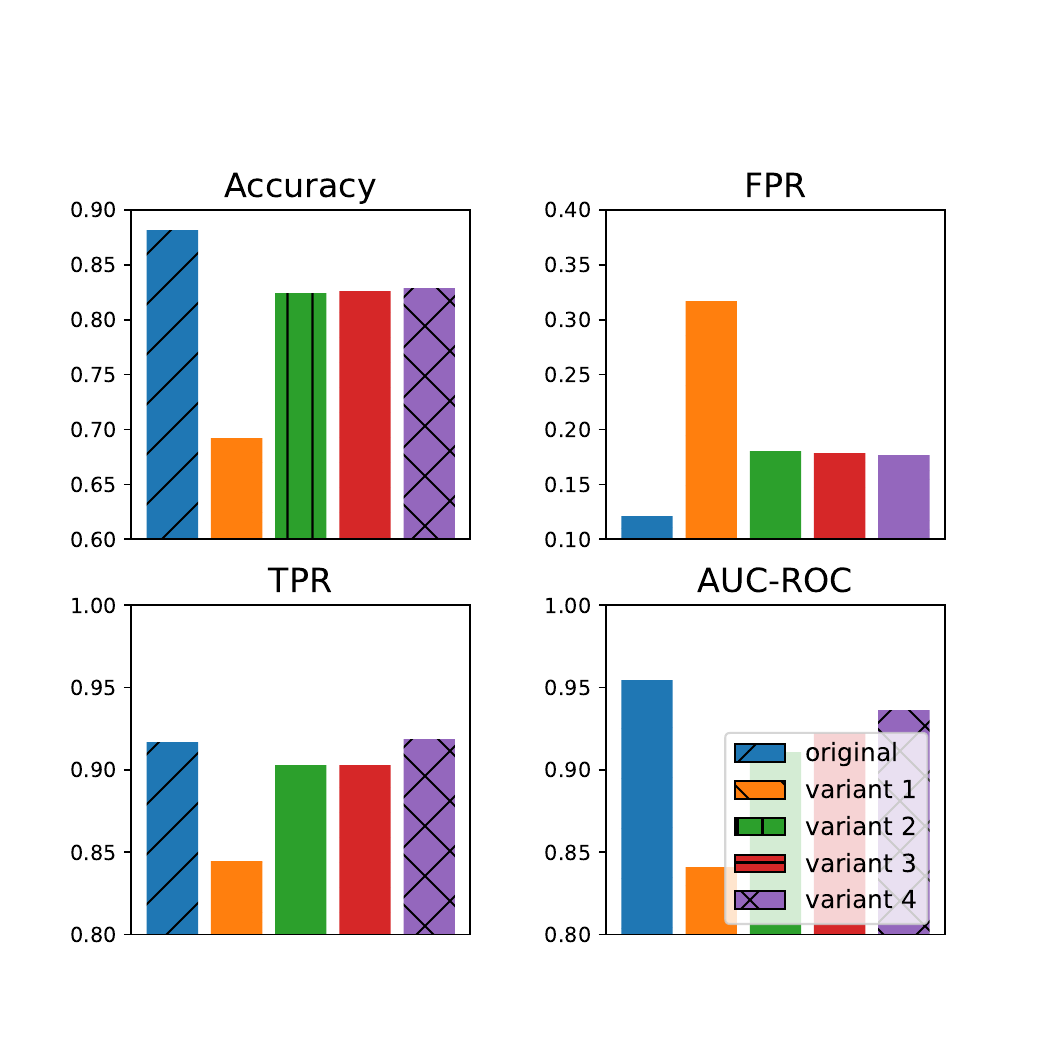}
    \caption{\bf Ablation study with GIN model.} 
    \label{fig:ablation_gin}
\end{figure}

\begin{figure}[t]
    \centering
    \includegraphics[width=0.9\linewidth]{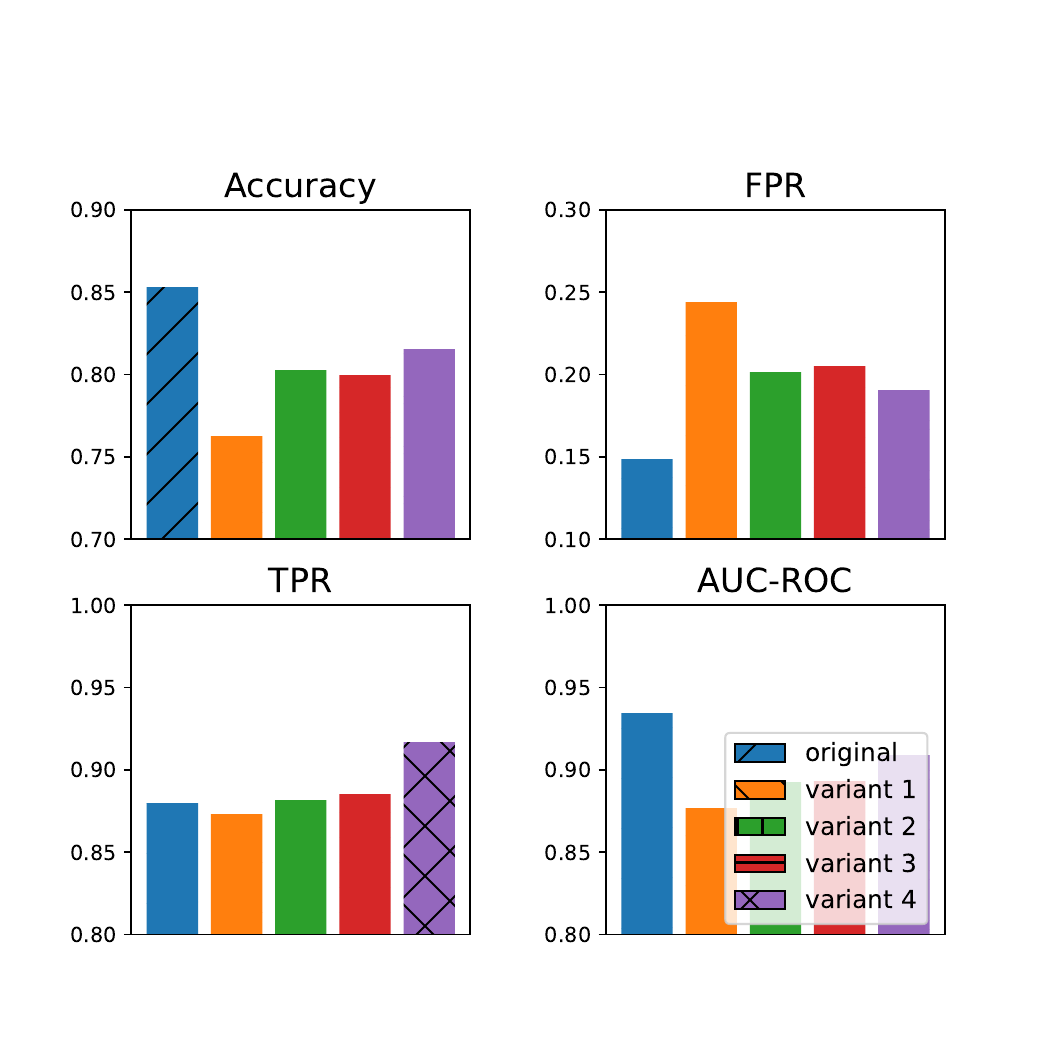}
    \caption{\bf Ablation study with GCN model.} 
    \label{fig:ablation_gcn}
\end{figure}

\begin{figure}[t]
    \centering
    \includegraphics[width=0.9\linewidth]{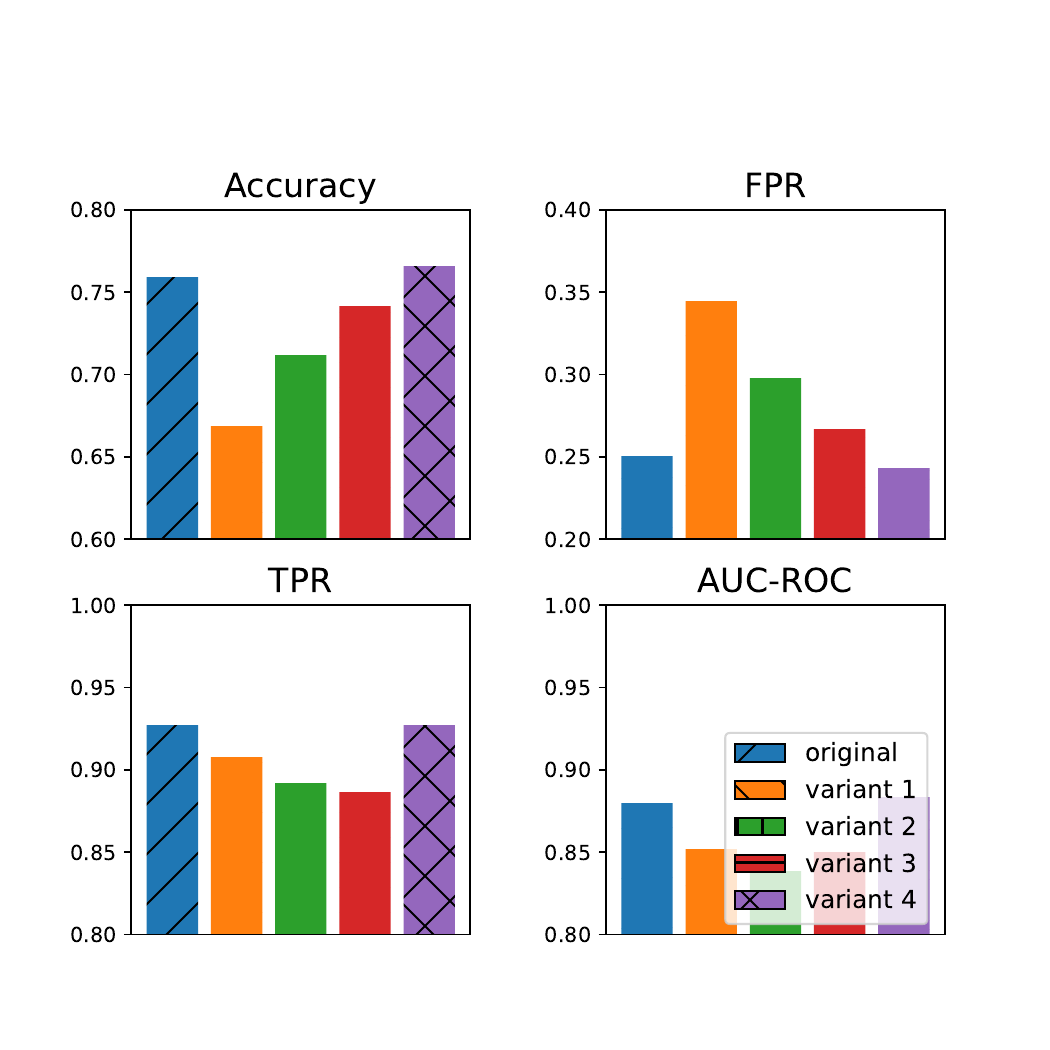}
    \caption{\bf Ablation study with MLP model.} 
    \label{fig:ablation_mlp}
\end{figure}
