# Supplementary material for: DeFiGuard: A Price Manipulation Detection Service in DeFi using Graph Neural Networks
Source: arXiv:2406.11157 source file (2024-06-17)
Supplement: Supplementary file 3 [file appendix_performance.tex]

\begin{figure*}[ht]
    \centering
    \includegraphics[width=1\linewidth]{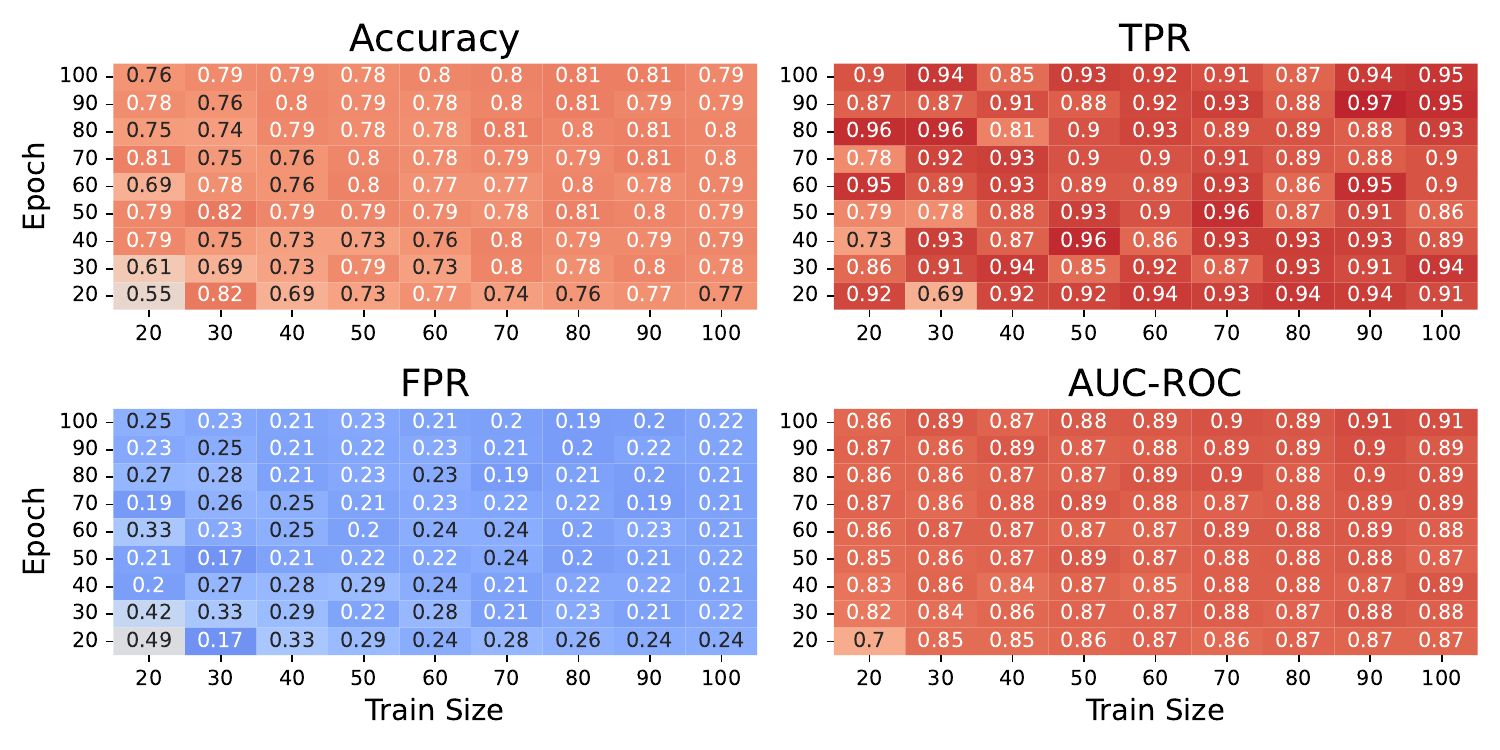}
    \caption{\bf The detailed performance of GCN.} 
    \label{fig:perf_gcn}
\end{figure*}

\begin{figure*}[ht]
    \centering
    \includegraphics[width=1\linewidth]{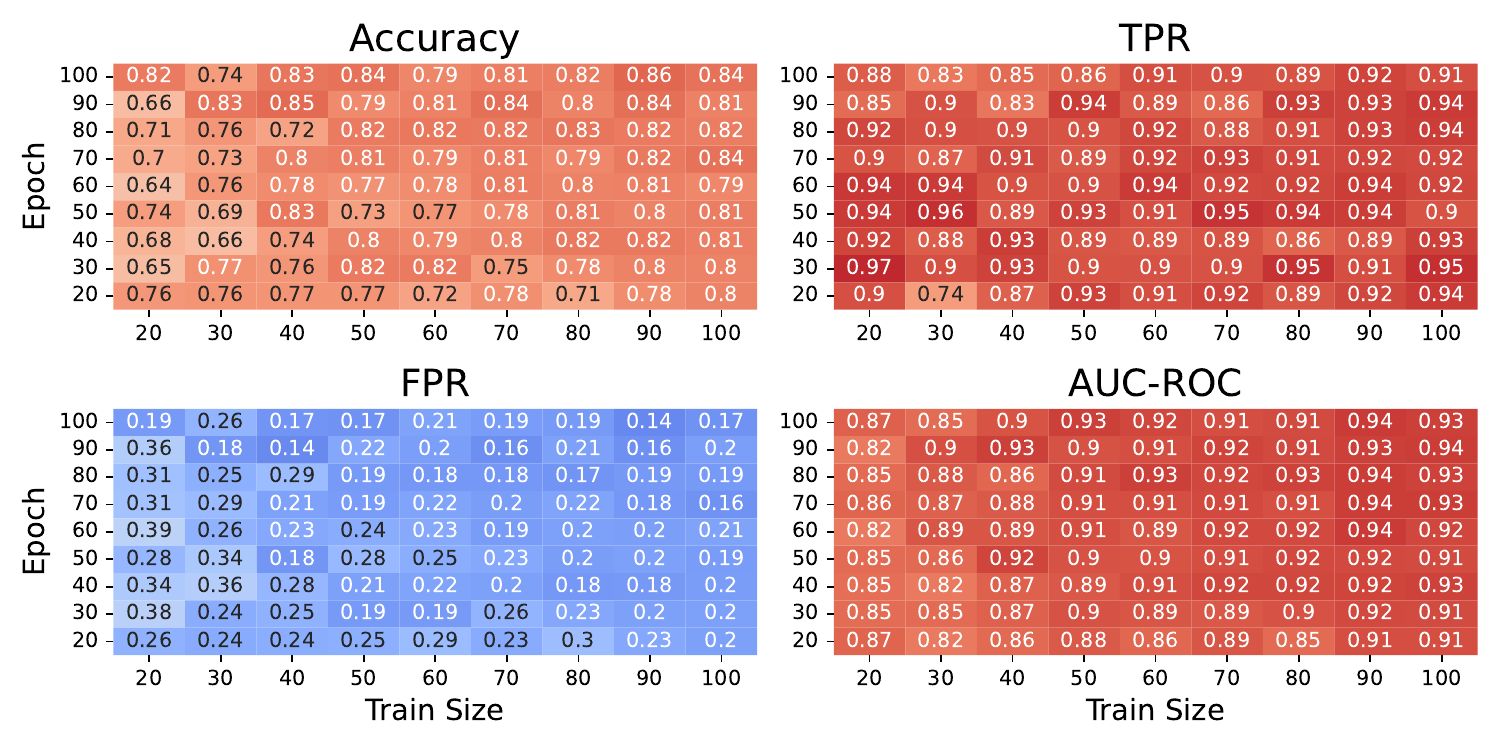}
    \caption{\bf The detailed performance of GAT.} 
    \label{fig:perf_gat}
\end{figure*}

\begin{figure*}[ht]
    \centering
    \includegraphics[width=1\linewidth]{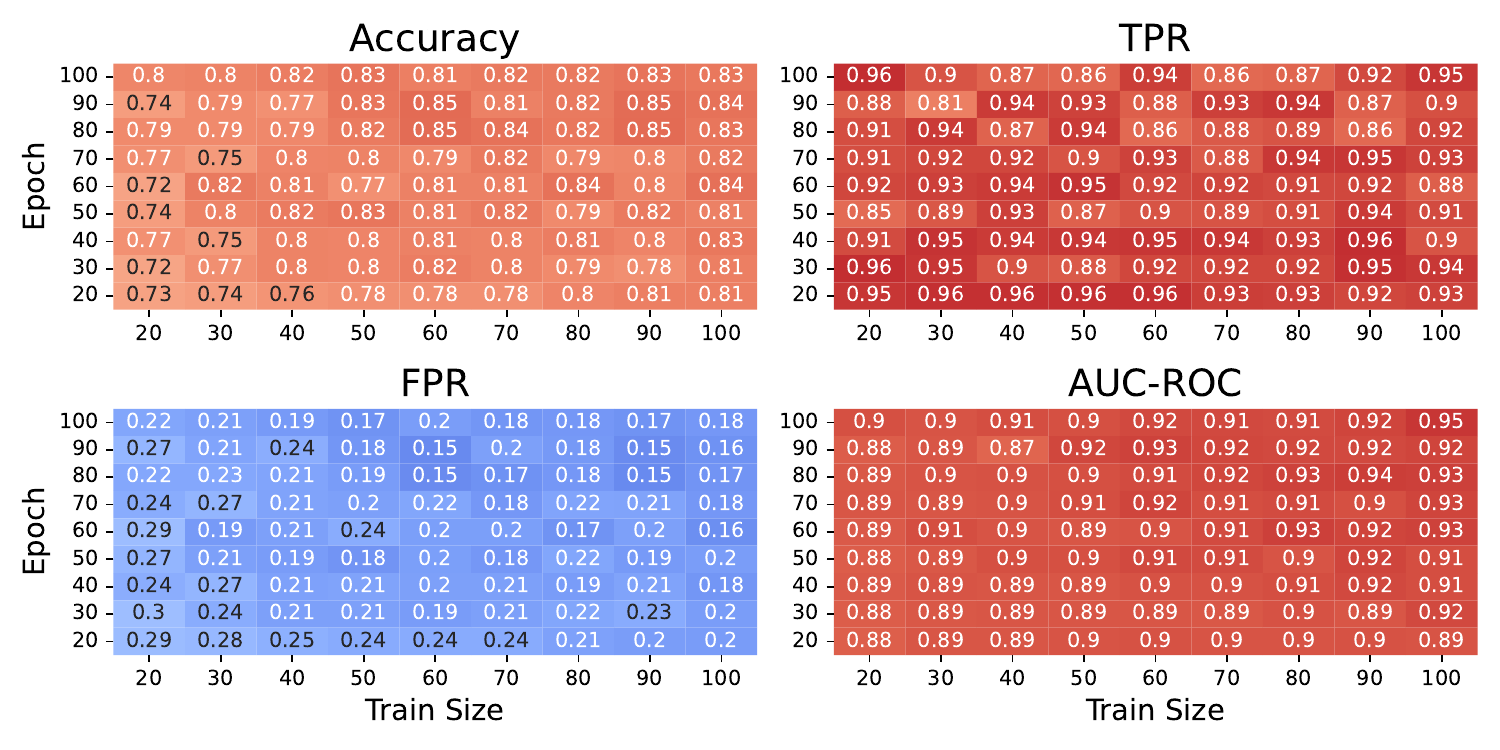}
    \caption{\bf The detailed performance of GIN.} 
    \label{fig:perf_gin}
\end{figure*}

\begin{figure*}[ht]
    \centering
    \includegraphics[width=1\linewidth]{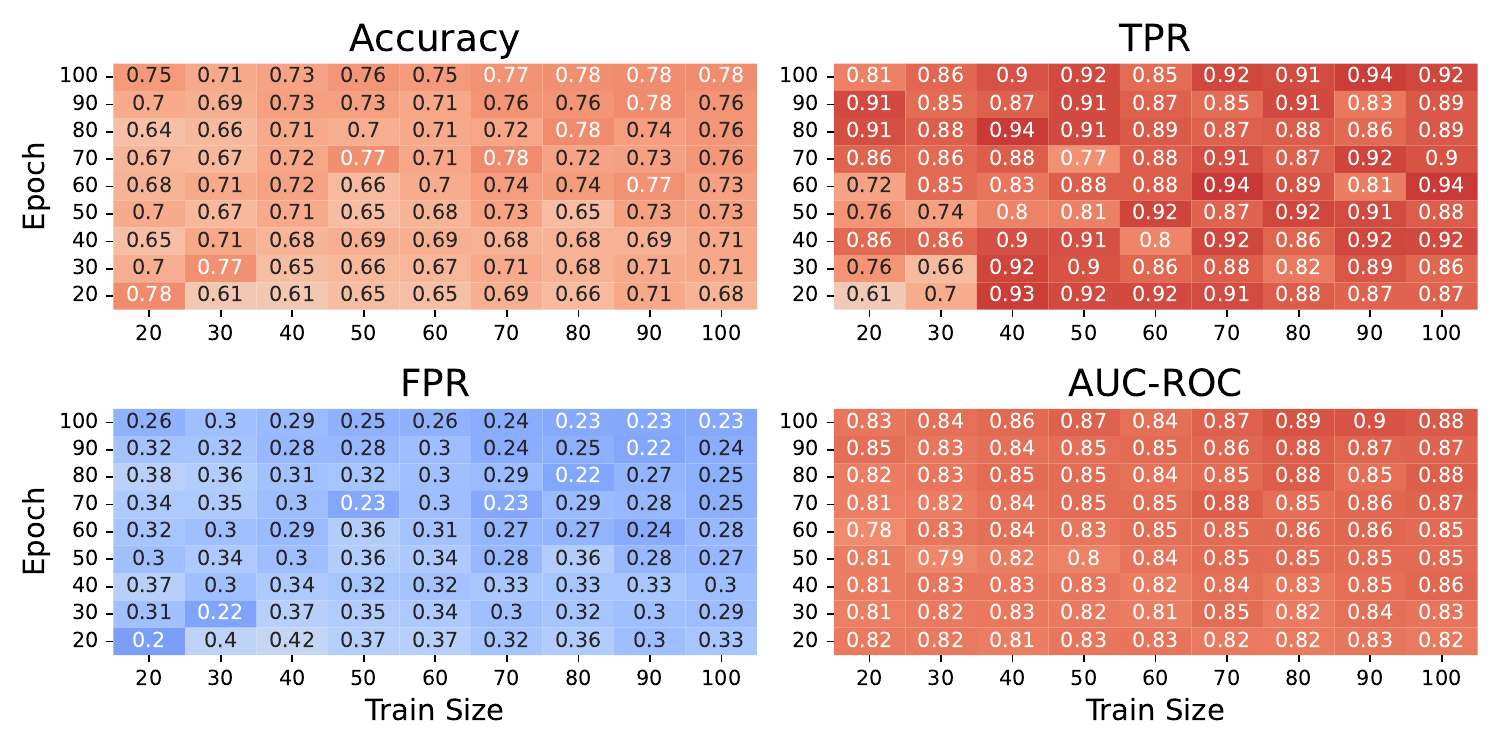}
    \caption{\bf The detailed performance of MLP.} 
    \label{fig:perf_mlp}
\end{figure*}
