# Supplementary material for: DeFiGuard: A Price Manipulation Detection Service in DeFi using Graph Neural Networks
Source: arXiv:2406.11157 source file (2024-06-17)
Supplement: Supplementary file 4 [file appendix_tx_comparison.tex]

% \begin{figure*}[t]
%     \centering
%     \begin{subfigure}{\textwidth}
%         \centering
%         \includegraphics[width=\linewidth]{pdf/malicious.png}
%         The transaction hash of the cash flow graph is 0x0fe2542079644e107cbf13690eb9c2c65963ccb79089ff96bfaf8dced2331c92.
%         \caption{The cash flow graph of a PMA transaction.}
%         \label{fig:tx_malicious}
%     \end{subfigure}
    
%     \begin{subfigure}{\textwidth}
%         \centering
%         \includegraphics[width=\linewidth]{pdf/benign.png}
%         The transaction hash of the cash flow graph is 0x0aad1020cb858d611339430310f9b679e7d7135454646e8e1f3b3802dbeaf0d0.
%         \caption{The cash flow graph of a non-PMA transaction.}
%         \label{fig:tx_benign}
%     \end{subfigure}
%     \caption{The comparison of the cash flow graph between PMA and non-PMA transactions.}
%     \label{fig:tx_comparison}
% \end{figure*}

% \begin{figure*}[t]
%     \centering
%         \centering
%         \includegraphics[width=0.8\linewidth]{pdf/malicious.png}
%         The transaction hash of the cash flow graph is 0x0fe2542079644e107cbf13690eb9c2c65963ccb79089ff96bfaf8dced2331c92.
%         \caption{The cash flow graph of a PMA transaction.}
% \end{figure*}
